# Supplementary material for: Effective and secure federated online learning to rank
Source: arXiv:2412.19069 source file (2024-12-26)
Supplement: Supplementary file 1 [file Appendix.tex]

% ***************************************************
% Appendix
% ***************************************************
\chapter{Appendix}

Write your appendix here. Following two are examples.

\section{Name of Appendix-1}

\section{Name of Appendix-2}
